# Supplementary material for: LPGNet: Link Private Graph Networks for Node Classification
Source: arXiv:2205.03105 source file (2022-09-07)
Supplement: Supplementary file 1 [file appendix-revision.tex]

\section{Addressing Suggestions for Revision}
\label{appdx:revision}

\paragraph*{S1: Add the formal DP proof and explain budget allocation}
We have explained both of them in detail in the Section~\ref{sec:ppandimpl}.

\paragraph*{S2: Fix issues in the Algorithms, writing issues and other formality issues}
We have rewritten the training and inference algorithms almost exactly as implemented in Algorithms~\ref{alg:lpgnet} and~\ref{alg:lpgnet_inf}, respectively. The privacy budget split is more evident in the algorithms now. Further, we have also added details of validation and reusing the degree vectors to them. The details of all edits we did for the pointed writing and formality issues are given in the Table~\ref{tab:other_fixes}.

\paragraph*{S3: Clarify what edge-DP does not protect against. Clarify why MLP is a reasonable baseline and why AUCs can be large. Clarify the connection between edge-DP and link-stealing attacks}
We add this discussion in Section~\ref{sec:discuss-eval}. We explain the difference between the attacks that predict edges because they are implied by a distribution of graphs learned by the GNN vs. the attacks that predict edges only when a GNN uses the edges from the training graph. We show why \baselineAttack, an example for the first kind, can achieve high AUCs even when edges are not used in Section~\ref{sec:discuss-eval}, paragraphs $1$ and $2$. We provide an example to show why \baselineAttack's AUC may not correspond to how much a GNN is leaking the edge information. Subsequently, we discuss why an increase in the attack AUC on GNNs with respect to \mlp is a better indicator for that.

\paragraph*{S4: An example where AUCs are not as large}
We show this on two datasets, one synthetic and one real-world dataset, in Section~\ref{sec:discuss-eval}. The best attack AUC is close to $0.5$ on \mlp and a maximum of around $0.73$ for \tool in the synthetic dataset and $0.6$ on the real-world dataset.

\paragraph*{S5: Please add a discussion on problems/datasets where edge-DP is not sufficient and possible mitigations}
We discuss this in Section~\ref{sec:discuss-eval}, last paragraph.

\begin{table*}[t]
    \centering
    \begin{tabular}{p{7cm}|p{7cm}}
        Suggestion & Our fix\\\hline
        The paper defines DP generally, but does not particularize for edge-DP. Is E is the set of edges or the number of edges (the paper uses E as both, but should be consistent about it) &  We write an additional paragraph to explain edge-DP in Section~\ref{sec:appl-setup}, last paragraph on Page 3, right side. We clear the confusion between E and $\Ec$ wherever necessary.\\\hline
        Is Laplace noise scalar? Do we need $\set{S}$ to be subset of $\set{R}$ & Yes, that is correct.\\\hline
        Does the paper only consider graphs that are undirected (symmetric adjacency matrix) and with unweighted edges? & Yes, that is correct and we mention it in Section~\ref{sec:appl-setup}, last paragraph on Page 3, right side. \\\hline
        The handling of the privacy budget is too informal in Algorithm 1: is $\epsilon_r$ always 0.01? Why not another parameter of the input? & We use it as a default value, however, it can be an input parameter. We have fixed it. \\\hline
        Convert $\tilde{E}$ to an integer in Algorithm 1 & We have fixed it. \\\hline
        Are MLPs trained sequentially? Clarify this. & We have added a footnote clarifying this in Section~\ref{sec:arch}.\\\hline
        The labels are not mentioned in Algorithm 2, further, which optimizer and loss function are you using? & We have fixed both of them in the algorithm.\\\hline
        Algorithm 3 has a bug with extra trainMLP & Yes, we have fixed it.\\\hline
        Why is \dpgcn with no privacy different from GCN & No it is not different. \\\hline
        Table 2 does not include \dpgcn & GCN is \dpgcn without DP. Nevertheless, we just wanted to show \tool's improvement in utility as \tool is the first of its kind ML model to learn from graphs even without DP. \\\hline
        % Label the axes in Figure 6 and consider explaining this figure better & We rephrase our previous ex\\\hline
        % Can we obtain privacy-utility plots for inductive & Need to figure out\\\hline
    \end{tabular}
    \caption{All the minor formality and writing issues}
    \label{tab:other_fixes} 
\end{table*}
