# Supplementary material for: LPGNet: Link Private Graph Networks for Node Classification
Source: arXiv:2205.03105 source file (2022-09-07)
Supplement: Supplementary file 2 [file ldp.tex]

\section{Extending to the LDP setup}
\label{appdx:ldpsetup}

\tool can also be extended for the federated setup where no data provider needs to be trusted with the graph. In this setup, each user (node) in the graph stores their neighbors locally. The data consumer can train \tool on its own servers while the users act as the data providers. Specifically, the data consumer will query every node for their noised degree vectors in each iteration by presenting the clusters from previous iteration. Users can noise their degree vectors locally by adding a noise of $Lap(0, \frac{1}{\epsilon})$ as adding or removing any of their edges may affect only one of their counts by $1$. However the total $\epsilon$ for an edge will still be $2\times\epsilon$ since each edge receives two such queries, one from each affected user.

\paragraph{Privacy risks in LDP setup} The data consumer gets access to all the intermediate logits, gradients, and the degree vectors throughout the training procedure which were not available in the centralized setup. This significantly increases the knowledge that can be used to infer the hidden edge structure. Further, if we do not assume that all users are honest then there is a significant risk for data poisoning attacks by the users~\cite{}. We provide the extension to LDP setup purely from the utility perspective given the recent rising interest in storing data locally. Similar to many existing works~\cite{} if we assume a setup where the users do not want to reveal their exact edges to train a GNN and are honestly following the DP protocol, then \tool may be useful in this setup. We leave studying the repercussions on privacy of the edges if we do not assume honest scenarios to future work.
