# Supplementary material for: LPGNet: Link Private Graph Networks for Node Classification
Source: arXiv:2205.03105 source file (2022-09-07)
Supplement: Supplementary file 3 [file Nl-1_2_Cora.tex]

\begin{table}[t]
\centering
\caption{Node classification results for the transductive setting using the micro-average F1 score on Cora Dataset.}

 \resizebox{\columnwidth}{!}{

\begin{tabular}{c c c c c c}
\toprule
Epsilon &  \mlp  & \toola & \toolb  & \gcn  &  \dpgcn \\\hline

1.0 & $0.6 \pm 0.0$ & $0.52 \pm 0.02$ & $ - $ & $0.81 \pm 0.0$ & $0.34 \pm 0.03$\\
2.0 & $0.6 \pm 0.0$ & $0.59 \pm 0.01$ & $0.56 \pm 0.02$ & $0.81 \pm 0.0$ & $0.35 \pm 0.02$\\
3.0 & $0.6 \pm 0.0$ & $0.63 \pm 0.02$ & $ - $ & $0.81 \pm 0.0$ & $0.35 \pm 0.02$\\
4.0 & $0.6 \pm 0.0$ & $0.65 \pm 0.02$ & $0.64 \pm 0.01$ & $0.81 \pm 0.0$ & $0.37 \pm 0.02$\\
5.0 & $0.6 \pm 0.0$ & $0.67 \pm 0.02$ & $ - $ & $0.81 \pm 0.0$ & $0.42 \pm 0.02$\\
6.0 & $0.6 \pm 0.0$ & $0.68 \pm 0.01$ & $0.68 \pm 0.01$ & $0.81 \pm 0.0$ & $0.53 \pm 0.02$\\
7.0 & $0.6 \pm 0.0$ & $0.68 \pm 0.01$ & $ - $ & $0.81 \pm 0.0$ & $0.66 \pm 0.01$\\
8.0 & $0.6 \pm 0.0$ & $0.69 \pm 0.02$ & $0.7 \pm 0.01$ & $0.81 \pm 0.0$ & $0.72 \pm 0.01$\\
9.0 & $0.6 \pm 0.0$ & $0.69 \pm 0.01$ & $ - $ & $0.81 \pm 0.0$ & $0.76 \pm 0.01$\\
10.0 & $0.6 \pm 0.0$ & $0.69 \pm 0.02$ & $0.71 \pm 0.01$ & $0.81 \pm 0.0$ & $0.78 \pm 0.01$\\
\hline
\end{tabular}
 }
\label{tab:cora-dp-ind}
\end{table}
