# Supplementary material for: LPGNet: Link Private Graph Networks for Node Classification
Source: arXiv:2205.03105 source file (2022-09-07)
Supplement: Supplementary file 4 [file Nl-1_2_PubMed.tex]

\begin{table}[t]
\centering
\caption{Node classification results for the transductive setting using the micro-average F1 score on Pubmed Dataset.}

 \resizebox{\columnwidth}{!}{

\begin{tabular}{c c c c c c}
\toprule
Epsilon &  \mlp  & \toola & \toolb  & \gcn  &  \dpgcn \\\hline

1.0 & $0.72 \pm 0.01$ & $0.71 \pm 0.01$ & $ - $ & $0.79 \pm 0.0$ & $0.55 \pm 0.02$\\
2.0 & $0.72 \pm 0.01$ & $0.73 \pm 0.01$ & $0.71 \pm 0.02$ & $0.79 \pm 0.0$ & $0.55 \pm 0.02$\\
3.0 & $0.72 \pm 0.01$ & $0.73 \pm 0.01$ & $ - $ & $0.79 \pm 0.0$ & $0.55 \pm 0.02$\\
4.0 & $0.72 \pm 0.01$ & $0.74 \pm 0.01$ & $0.73 \pm 0.01$ & $0.79 \pm 0.0$ & $0.55 \pm 0.02$\\
5.0 & $0.72 \pm 0.01$ & $0.74 \pm 0.0$ & $ - $ & $0.79 \pm 0.0$ & $0.55 \pm 0.02$\\
6.0 & $0.72 \pm 0.01$ & $0.74 \pm 0.01$ & $0.74 \pm 0.01$ & $0.79 \pm 0.0$ & $0.56 \pm 0.02$\\
7.0 & $0.72 \pm 0.01$ & $0.74 \pm 0.0$ & $ - $ & $0.79 \pm 0.0$ & $0.59 \pm 0.02$\\
8.0 & $0.72 \pm 0.01$ & $0.74 \pm 0.0$ & $0.74 \pm 0.01$ & $0.79 \pm 0.0$ & $0.64 \pm 0.02$\\
9.0 & $0.72 \pm 0.01$ & $0.74 \pm 0.0$ & $ - $ & $0.79 \pm 0.0$ & $0.69 \pm 0.02$\\
10.0 & $0.72 \pm 0.01$ & $0.74 \pm 0.0$ & $0.75 \pm 0.01$ & $0.79 \pm 0.0$ & $0.73 \pm 0.02$\\
\hline
\end{tabular}
 }
\label{tab:pubmed-dp-ind}
\end{table}
