# Supplementary material for: LPGNet: Link Private Graph Networks for Node Classification
Source: arXiv:2205.03105 source file (2022-09-07)
Supplement: Supplementary file 5 [file Nl1_2-Citeseer.tex]

\begin{table}[t]
\centering
\caption{Node classification results for the transductive setting using the micro-average F1 score on Citeseer Dataset.}

 \resizebox{\columnwidth}{!}{

\begin{tabular}{c c c c c c}
\toprule
Epsilon &  \mlp  & \toola & \toolb  & \gcn  &  \dpgcn \\\hline

1.0 & $0.6 \pm 0.01$ & $0.58 \pm 0.02$ & $ - $ & $0.72 \pm 0.0$ & $0.36 \pm 0.02$\\
2.0 & $0.6 \pm 0.01$ & $0.62 \pm 0.01$ & $0.55 \pm 0.02$ & $0.72 \pm 0.0$ & $0.36 \pm 0.02$\\
3.0 & $0.6 \pm 0.01$ & $0.63 \pm 0.01$ & $ - $ & $0.72 \pm 0.0$ & $0.37 \pm 0.01$\\
4.0 & $0.6 \pm 0.01$ & $0.64 \pm 0.01$ & $0.62 \pm 0.01$ & $0.72 \pm 0.0$ & $0.38 \pm 0.02$\\
5.0 & $0.6 \pm 0.01$ & $0.64 \pm 0.01$ & $ - $ & $0.72 \pm 0.0$ & $0.41 \pm 0.02$\\
6.0 & $0.6 \pm 0.01$ & $0.64 \pm 0.01$ & $0.64 \pm 0.01$ & $0.72 \pm 0.0$ & $0.46 \pm 0.02$\\
7.0 & $0.6 \pm 0.01$ & $0.64 \pm 0.01$ & $ - $ & $0.72 \pm 0.0$ & $0.55 \pm 0.02$\\
8.0 & $0.6 \pm 0.01$ & $0.65 \pm 0.01$ & $0.65 \pm 0.01$ & $0.72 \pm 0.0$ & $0.62 \pm 0.02$\\
9.0 & $0.6 \pm 0.01$ & $0.65 \pm 0.01$ & $ - $ & $0.72 \pm 0.0$ & $0.67 \pm 0.01$\\
10.0 & $0.6 \pm 0.01$ & $0.65 \pm 0.01$ & $0.65 \pm 0.01$ & $0.72 \pm 0.0$ & $0.69 \pm 0.01$\\
\hline
\end{tabular}
 }
\label{tab:citeseer-dp-ind}
\end{table}
