# Supplementary material for: LPGNet: Link Private Graph Networks for Node Classification
Source: arXiv:2205.03105 source file (2022-09-07)
Supplement: Supplementary file 7 [file Nl_1_2_Facebook_page.tex]

\begin{table}[t]
\centering
\caption{Node classification results for the transductive setting using the micro-average F1 score on Facebook Dataset.}

 \resizebox{\columnwidth}{!}{

\begin{tabular}{c c c c c c}
\toprule
Epsilon &  \mlp  & \toola & \toolb  & \gcn  &  \dpgcn \\\hline

1.0 & $0.74 \pm 0.01$ & $0.78 \pm 0.01$ & $ - $ & $0.93 \pm 0.0$ & $0.3 \pm 0.01$\\
2.0 & $0.74 \pm 0.01$ & $0.8 \pm 0.01$ & $0.8 \pm 0.01$ & $0.93 \pm 0.0$ & $0.3 \pm 0.01$\\
3.0 & $0.74 \pm 0.01$ & $0.81 \pm 0.01$ & $ - $ & $0.93 \pm 0.0$ & $0.3 \pm 0.01$\\
4.0 & $0.74 \pm 0.01$ & $0.82 \pm 0.01$ & $0.83 \pm 0.01$ & $0.93 \pm 0.0$ & $0.3 \pm 0.01$\\
5.0 & $0.74 \pm 0.01$ & $0.82 \pm 0.01$ & $ - $ & $0.93 \pm 0.0$ & $0.35 \pm 0.01$\\
6.0 & $0.74 \pm 0.01$ & $0.82 \pm 0.01$ & $0.85 \pm 0.01$ & $0.93 \pm 0.0$ & $0.47 \pm 0.03$\\
7.0 & $0.74 \pm 0.01$ & $0.82 \pm 0.01$ & $ - $ & $0.93 \pm 0.0$ & $0.63 \pm 0.01$\\
8.0 & $0.74 \pm 0.01$ & $0.83 \pm 0.01$ & $0.85 \pm 0.01$ & $0.93 \pm 0.0$ & $0.74 \pm 0.01$\\
9.0 & $0.74 \pm 0.01$ & $0.83 \pm 0.01$ & $ - $ & $0.93 \pm 0.0$ & $0.81 \pm 0.01$\\
10.0 & $0.74 \pm 0.01$ & $0.83 \pm 0.01$ & $0.86 \pm 0.01$ & $0.93 \pm 0.0$ & $0.85 \pm 0.01$\\
\hline
\end{tabular}
 }
\label{tab:facebook-dp-ind}
\end{table}
