# Supplementary material for: LPGNet: Link Private Graph Networks for Node Classification
Source: arXiv:2205.03105 source file (2022-09-07)
Supplement: Supplementary file 9 [file Nl_1_2_TwitchENGB.tex]

\begin{table}[t]
\centering
\caption{Node classification results for the inductive setting using the rare F1 score on Twitch-ENGB Dataset.}

 \resizebox{\columnwidth}{!}{

\begin{tabular}{c c c c c c}
\toprule
Epsilon &  \mlp  & \toola & \toolb  & \gcn  &  \dpgcn \\\hline

1.0 & $0.6 \pm 0.0$ & $0.6 \pm 0.0$ & $ - $ & $0.6 \pm 0.0$ & $0.6 \pm 0.01$\\
2.0 & $0.6 \pm 0.0$ & $0.6 \pm 0.0$ & $0.6 \pm 0.0$ & $0.6 \pm 0.0$ & $0.6 \pm 0.01$\\
3.0 & $0.6 \pm 0.0$ & $0.6 \pm 0.0$ & $ - $ & $0.6 \pm 0.0$ & $0.6 \pm 0.01$\\
4.0 & $0.6 \pm 0.0$ & $0.6 \pm 0.0$ & $0.6 \pm 0.0$ & $0.6 \pm 0.0$ & $0.6 \pm 0.01$\\
5.0 & $0.6 \pm 0.0$ & $0.6 \pm 0.0$ & $ - $ & $0.6 \pm 0.0$ & $0.6 \pm 0.01$\\
6.0 & $0.6 \pm 0.0$ & $0.6 \pm 0.0$ & $0.6 \pm 0.0$ & $0.6 \pm 0.0$ & $0.6 \pm 0.01$\\
7.0 & $0.6 \pm 0.0$ & $0.6 \pm 0.0$ & $ - $ & $0.6 \pm 0.0$ & $0.6 \pm 0.01$\\
8.0 & $0.6 \pm 0.0$ & $0.6 \pm 0.0$ & $0.6 \pm 0.0$ & $0.6 \pm 0.0$ & $0.6 \pm 0.01$\\
9.0 & $0.6 \pm 0.0$ & $0.6 \pm 0.01$ & $ - $ & $0.6 \pm 0.0$ & $0.6 \pm 0.01$\\
10.0 & $0.6 \pm 0.0$ & $0.6 \pm 0.01$ & $0.6 \pm 0.0$ & $0.6 \pm 0.0$ & $0.6 \pm 0.0$\\
\hline
\end{tabular}
 }
\label{tab:engb-dp-ind}
\end{table}
