# Supplementary material for: LPGNet: Link Private Graph Networks for Node Classification
Source: arXiv:2205.03105 source file (2022-09-07)
Supplement: Supplementary file 13 [file attack.tex]

\begin{table*}[th!]
   \centering
\caption{Attack in Transductive Setting}

   \resizebox{\textwidth}{!}{
%\toprule
\begin{tabular}{c c c c c c c c c c } 
     \toprule       Model & Epsilon   & \multicolumn{2}{c}{Citeseer}  & \multicolumn{2}{c}{Cora}  & \multicolumn{2}{c}{Facebook}  & \multicolumn{2}{c}{Pubmed}               \\
     \hline 
                  &           &   \baselineAttack & \sotaAttack                 &   \baselineAttack & \sotaAttack              &   \baselineAttack & \sotaAttack                &   \baselineAttack & \sotaAttack                             \\
    \hline
\mlp
& $0.0$& $0.78 \pm 0.02$& $0.50 \pm 0.00$& $0.74 \pm 0.02$& $0.50 \pm 0.00$& $0.81 \pm 0.02$& $0.50 \pm 0.00$& $0.75 \pm 0.02$& $0.50 \pm 0.00$\\

\hline
\gcn
& $0.0$& $0.96 \pm 0.00$& $1.00 \pm 0.00$& $0.94 \pm 0.01$& $1.00 \pm 0.00$& $0.88 \pm 0.01$& $1.00 \pm 0.00$& $0.87 \pm 0.01$& $1.00 \pm 0.00$\\

\hline
\multirow{11}{*}{\dpgcn}
& $1.0$& $0.61 \pm 0.03$& $0.50 \pm 0.00$& $0.58 \pm 0.02$& $0.50 \pm 0.00$& $0.50 \pm 0.01$& $0.50 \pm 0.00$& $0.58 \pm 0.02$& $0.50 \pm 0.00$\\

& $2.0$& $0.62 \pm 0.03$& $0.50 \pm 0.00$& $0.60 \pm 0.01$& $0.50 \pm 0.00$& $0.50 \pm 0.02$& $0.50 \pm 0.00$& $0.60 \pm 0.01$& $0.50 \pm 0.00$\\

& $3.0$& $0.62 \pm 0.03$& $0.51 \pm 0.00$& $0.59 \pm 0.01$& $0.51 \pm 0.00$& $0.51 \pm 0.02$& $0.50 \pm 0.00$& $0.58 \pm 0.02$& $0.50 \pm 0.00$\\

& $4.0$& $0.64 \pm 0.02$& $0.52 \pm 0.00$& $0.62 \pm 0.02$& $0.53 \pm 0.00$& $0.50 \pm 0.02$& $0.51 \pm 0.00$& $0.60 \pm 0.03$& $0.50 \pm 0.00$\\

& $5.0$& $0.67 \pm 0.02$& $0.55 \pm 0.01$& $0.67 \pm 0.02$& $0.59 \pm 0.01$& $0.54 \pm 0.01$& $0.54 \pm 0.01$& $0.61 \pm 0.02$& $0.51 \pm 0.00$\\

& $6.0$& $0.73 \pm 0.02$& $0.63 \pm 0.01$& $0.76 \pm 0.01$& $0.69 \pm 0.01$& $0.63 \pm 0.02$& $0.66 \pm 0.02$& $0.62 \pm 0.02$& $0.54 \pm 0.00$\\

& $7.0$& $0.81 \pm 0.02$& $0.75 \pm 0.01$& $0.84 \pm 0.01$& $0.82 \pm 0.00$& $0.72 \pm 0.01$& $0.82 \pm 0.01$& $0.66 \pm 0.02$& $0.59 \pm 0.01$\\

& $8.0$& $0.88 \pm 0.01$& $0.85 \pm 0.01$& $0.88 \pm 0.01$& $0.90 \pm 0.00$& $0.79 \pm 0.02$& $0.92 \pm 0.01$& $0.73 \pm 0.01$& $0.70 \pm 0.01$\\

& $9.0$& $0.92 \pm 0.01$& $0.91 \pm 0.01$& $0.9 \pm 0.01$& $0.95 \pm 0.00$& $0.83 \pm 0.01$& $0.96 \pm 0.01$& $0.78 \pm 0.03$& $0.82 \pm 0.01$\\

& $10.0$& $0.93 \pm 0.01$& $0.95 \pm 0.01$& $0.92 \pm 0.01$& $0.97 \pm 0.00$& $0.85 \pm 0.01$& $0.98 \pm 0.00$& $0.81 \pm 0.01$& $0.89 \pm 0.01$\\

\hline
\multirow{11}{*}{\toola}
& $0.0$& $0.86 \pm 0.01$& $0.50 \pm 0.00$& $0.87 \pm 0.01$& $0.50 \pm 0.00$& $0.85 \pm 0.01$& $0.50 \pm 0.00$& $0.80 \pm 0.01$& $0.50 \pm 0.00$\\

& $1.0$& $0.77 \pm 0.03$& $0.50 \pm 0.00$& $0.72 \pm 0.02$& $0.50 \pm 0.00$& $0.82 \pm 0.01$& $0.50 \pm 0.00$& $0.76 \pm 0.01$& $0.50 \pm 0.00$\\

& $2.0$& $0.81 \pm 0.01$& $0.50 \pm 0.00$& $0.78 \pm 0.02$& $0.50 \pm 0.00$& $0.83 \pm 0.01$& $0.50 \pm 0.00$& $0.77 \pm 0.00$& $0.50 \pm 0.00$\\

& $3.0$& $0.83 \pm 0.02$& $0.50 \pm 0.00$& $0.82 \pm 0.01$& $0.50 \pm 0.00$& $0.84 \pm 0.01$& $0.50 \pm 0.00$& $0.79 \pm 0.00$& $0.50 \pm 0.00$\\

& $4.0$& $0.84 \pm 0.02$& $0.50 \pm 0.00$& $0.83 \pm 0.01$& $0.50 \pm 0.00$& $0.85 \pm 0.01$& $0.50 \pm 0.00$& $0.78 \pm 0.02$& $0.50 \pm 0.00$\\

& $5.0$& $0.84 \pm 0.01$& $0.50 \pm 0.00$& $0.85 \pm 0.02$& $0.50 \pm 0.00$& $0.84 \pm 0.01$& $0.50 \pm 0.00$& $0.78 \pm 0.01$& $0.50 \pm 0.00$\\

& $6.0$& $0.84 \pm 0.02$& $0.50 \pm 0.00$& $0.85 \pm 0.01$& $0.50 \pm 0.00$& $0.85 \pm 0.01$& $0.50 \pm 0.00$& $0.79 \pm 0.01$& $0.43 \pm 0.01$\\

& $7.0$& $0.86 \pm 0.01$& $0.50 \pm 0.00$& $0.85 \pm 0.01$& $0.50 \pm 0.00$& $0.85 \pm 0.02$& $0.50 \pm 0.00$& $0.79 \pm 0.01$& $0.50 \pm 0.00$\\

& $8.0$& $0.86 \pm 0.01$& $0.50 \pm 0.00$& $0.86 \pm 0.01$& $0.50 \pm 0.00$& $0.85 \pm 0.01$& $0.50 \pm 0.00$& $0.78 \pm 0.02$& $0.50 \pm 0.00$\\

& $9.0$& $0.86 \pm 0.01$& $0.50 \pm 0.00$& $0.85 \pm 0.01$& $0.50 \pm 0.00$& $0.85 \pm 0.01$& $0.50 \pm 0.00$& $0.80 \pm 0.01$& $0.50 \pm 0.00$\\

& $10.0$& $0.85 \pm 0.01$& $0.50 \pm 0.00$& $0.86 \pm 0.01$& $0.50 \pm 0.00$& $0.85 \pm 0.01$& $0.50 \pm 0.00$& $0.79 \pm 0.02$& $0.50 \pm 0.00$\\

\hline
\multirow{10}{*}{\toolb}
& $0.0$& $0.89 \pm 0.01$& $0.50 \pm 0.00$& $0.88 \pm 0.01$& $0.50 \pm 0.00$& $0.86 \pm 0.01$& $0.50 \pm 0.00$& $0.82 \pm 0.01$& $0.50 \pm 0.00$\\

& $1.0$& $0.75 \pm 0.02$& $0.50 \pm 0.00$& $0.74 \pm 0.01$& $0.50 \pm 0.00$& $0.83 \pm 0.01$& $0.50 \pm 0.00$& $0.75 \pm 0.01$& $0.50 \pm 0.00$\\

& $2.0$& $0.81 \pm 0.02$& $0.50 \pm 0.00$& $0.81 \pm 0.01$& $0.50 \pm 0.00$& $0.84 \pm 0.02$& $0.50 \pm 0.00$& $0.78 \pm 0.01$& $0.50 \pm 0.00$\\

& $3.0$& $0.83 \pm 0.02$& $0.50 \pm 0.00$& $0.84 \pm 0.01$& $0.50 \pm 0.00$& $0.84 \pm 0.01$& $0.50 \pm 0.00$& $0.79 \pm 0.01$& $0.50 \pm 0.00$\\

& $4.0$& $0.87 \pm 0.01$& $0.50 \pm 0.00$& $0.86 \pm 0.01$& $0.50 \pm 0.00$& $0.85 \pm 0.01$& $0.50 \pm 0.00$& $0.80 \pm 0.00$& $0.50 \pm 0.00$\\

& $5.0$& $0.86 \pm 0.01$& $0.50 \pm 0.00$& $0.85 \pm 0.01$& $0.50 \pm 0.00$& $0.85 \pm 0.01$& $0.50 \pm 0.00$& $0.80 \pm 0.01$& $0.50 \pm 0.00$\\

& $6.0$& $0.87 \pm 0.01$& $0.50 \pm 0.00$& $0.86 \pm 0.01$& $0.50 \pm 0.00$& $0.85 \pm 0.01$& $0.50 \pm 0.00$& $0.79 \pm 0.02$& $0.50 \pm 0.00$\\

& $7.0$& $0.87 \pm 0.01$& $0.50 \pm 0.00$& $0.86 \pm 0.01$& $0.50 \pm 0.00$& $0.84 \pm 0.01$& $0.50 \pm 0.00$& $0.80 \pm 0.01$& $0.50 \pm 0.00$\\

& $8.0$& $0.88 \pm 0.01$& $0.50 \pm 0.00$& $0.86 \pm 0.01$& $0.50 \pm 0.00$& $0.85 \pm 0.02$& $0.50 \pm 0.00$& $0.81 \pm 0.01$& $0.50 \pm 0.00$\\

& $9.0$& $0.87 \pm 0.01$& $0.50 \pm 0.00$& $0.87 \pm 0.01$& $0.50 \pm 0.00$& $0.85 \pm 0.01$& $0.50 \pm 0.00$& $0.80 \pm 0.01$& $0.50 \pm 0.00$\\

& $10.0$& $0.87 \pm 0.01$& $0.50 \pm 0.00$& $0.87 \pm 0.01$& $0.50 \pm 0.00$& $0.86 \pm 0.01$& $0.50 \pm 0.00$& $0.80 \pm 0.01$& $0.50 \pm 0.00$\\

\hline
\end{tabular}
       }
\label{tab:hyperparameters}
       \end{table*}
