# Supplementary material for: LPGNet: Link Private Graph Networks for Node Classification
Source: arXiv:2205.03105 source file (2022-09-07)
Supplement: Supplementary file 14 [file attack_engb.tex]

\begin{table*}[t]
   \centering
\caption{Attack Table in Inductive Setting in Twitch-ENGB Dataset.}

   \resizebox{\textwidth}{!}{

\begin{tabular}{c c c c c c c c c c c c c} 
            Model & Epsilon   & \multicolumn{2}{c}{\baselineAttack}  & \multicolumn{2}{c}{\sotaAttack} \\
    \hline 
                  &           &  lo   & hi & baseline                 &   lo & hi & baseline    \\
    \hline
GCN
& $0$& $0.65\pm0.08$& $0.55\pm0.02$&$0.56\pm0.01$&$1.0\pm0.0$&$0.99\pm0.0$&$1.0\pm0.0$\\

\hline
\multirow{10}{*}{DPGCN}
& $1$& $0.57\pm0.09$& $0.51\pm0.01$&$0.49\pm0.02$&$0.51\pm0.03$&$0.5\pm0.0$&$0.5\pm0.0$\\

& $2$& $0.56\pm0.08$& $0.51\pm0.01$&$0.47\pm0.03$&$0.48\pm0.02$&$0.51\pm0.01$&$0.5\pm0.0$\\

& $3$& $0.55\pm0.08$& $0.5\pm0.01$&$0.47\pm0.01$&$0.47\pm0.01$&$0.52\pm0.0$&$0.51\pm0.01$\\

& $4$& $0.53\pm0.1$& $0.51\pm0.02$&$0.48\pm0.05$&$0.53\pm0.05$&$0.55\pm0.01$&$0.55\pm0.02$\\

& $5$& $0.49\pm0.07$& $0.52\pm0.01$&$0.49\pm0.01$&$0.56\pm0.06$&$0.64\pm0.01$&$0.64\pm0.03$\\

& $6$& $0.47\pm0.08$& $0.52\pm0.02$&$0.5\pm0.03$&$0.63\pm0.09$&$0.78\pm0.01$&$0.77\pm0.02$\\

& $7$& $0.57\pm0.05$& $0.54\pm0.01$&$0.52\pm0.03$&$0.79\pm0.07$&$0.9\pm0.01$&$0.89\pm0.01$\\

& $8$& $0.49\pm0.07$& $0.54\pm0.01$&$0.51\pm0.04$&$0.87\pm0.07$&$0.95\pm0.0$&$0.95\pm0.01$\\

& $9$& $0.56\pm0.03$& $0.54\pm0.01$&$0.52\pm0.02$&$0.92\pm0.05$&$0.96\pm0.0$&$0.97\pm0.0$\\

& $10$& $0.58\pm0.03$& $0.54\pm0.02$&$0.53\pm0.01$&$0.94\pm0.05$&$0.98\pm0.0$&$0.98\pm0.01$\\

\hline
\multirow{11}{*}{\toola}
& $0$& $0.49\pm0.03$& $0.52\pm0.01$&$0.49\pm0.03$&$0.5\pm0.0$&$0.5\pm0.0$&$0.5\pm0.0$\\

& $1$& $0.49\pm0.1$& $0.51\pm0.0$&$0.48\pm0.02$&$0.5\pm0.0$&$0.5\pm0.0$&$0.5\pm0.0$\\

& $2$& $0.52\pm0.09$& $0.51\pm0.01$&$0.47\pm0.02$&$0.5\pm0.0$&$0.5\pm0.0$&$0.5\pm0.0$\\

& $3$& $0.51\pm0.09$& $0.52\pm0.01$&$0.49\pm0.02$&$0.5\pm0.0$&$0.5\pm0.0$&$0.5\pm0.0$\\

& $4$& $0.46\pm0.08$& $0.51\pm0.01$&$0.46\pm0.04$&$0.5\pm0.0$&$0.5\pm0.0$&$0.5\pm0.0$\\

& $5$& $0.51\pm0.08$& $0.51\pm0.01$&$0.49\pm0.02$&$0.5\pm0.0$&$0.5\pm0.0$&$0.5\pm0.0$\\

& $6$& $0.52\pm0.12$& $0.51\pm0.01$&$0.49\pm0.03$&$0.5\pm0.0$&$0.5\pm0.0$&$0.5\pm0.0$\\

& $7$& $0.49\pm0.07$& $0.52\pm0.0$&$0.5\pm0.02$&$0.5\pm0.0$&$0.5\pm0.0$&$0.5\pm0.0$\\

& $8$& $0.49\pm0.12$& $0.51\pm0.0$&$0.49\pm0.03$&$0.5\pm0.0$&$0.5\pm0.0$&$0.5\pm0.0$\\

& $9$& $0.5\pm0.08$& $0.51\pm0.0$&$0.5\pm0.02$&$0.5\pm0.0$&$0.5\pm0.0$&$0.5\pm0.0$\\

& $10$& $0.47\pm0.06$& $0.52\pm0.01$&$0.49\pm0.03$&$0.5\pm0.0$&$0.5\pm0.0$&$0.5\pm0.0$\\

\hline
\multirow{11}{*}{\toolb}
& $0$& $0.5\pm0.03$& $0.5\pm0.01$&$0.48\pm0.02$&$0.5\pm0.0$&$0.5\pm0.0$&$0.5\pm0.0$\\

& $1$& $0.48\pm0.09$& $0.51\pm0.01$&$0.48\pm0.02$&$0.5\pm0.0$&$0.5\pm0.0$&$0.5\pm0.0$\\

& $2$& $0.51\pm0.05$& $0.51\pm0.01$&$0.47\pm0.02$&$0.5\pm0.0$&$0.5\pm0.0$&$0.5\pm0.0$\\

& $3$& $0.47\pm0.06$& $0.51\pm0.0$&$0.48\pm0.03$&$0.5\pm0.0$&$0.5\pm0.0$&$0.5\pm0.0$\\

& $4$& $0.53\pm0.06$& $0.52\pm0.01$&$0.48\pm0.02$&$0.5\pm0.0$&$0.5\pm0.0$&$0.5\pm0.0$\\

& $5$& $0.51\pm0.05$& $0.51\pm0.0$&$0.49\pm0.02$&$0.5\pm0.0$&$0.5\pm0.0$&$0.5\pm0.0$\\

& $6$& $0.48\pm0.08$& $0.51\pm0.0$&$0.47\pm0.02$&$0.5\pm0.0$&$0.5\pm0.0$&$0.5\pm0.0$\\

& $7$& $0.52\pm0.03$& $0.51\pm0.01$&$0.49\pm0.04$&$0.5\pm0.0$&$0.5\pm0.0$&$0.5\pm0.0$\\

& $8$& $0.47\pm0.05$& $0.52\pm0.01$&$0.48\pm0.01$&$0.5\pm0.0$&$0.5\pm0.0$&$0.5\pm0.0$\\

& $9$& $0.47\pm0.09$& $0.51\pm0.0$&$0.48\pm0.02$&$0.5\pm0.0$&$0.5\pm0.0$&$0.5\pm0.0$\\

& $10$& $0.47\pm0.07$& $0.52\pm0.01$&$0.48\pm0.02$&$0.5\pm0.0$&$0.5\pm0.0$&$0.5\pm0.0$\\

\hline
\multirow{11}{*}{\toolc}
& $0$& $0.52\pm0.04$& $0.52\pm0.01$&$0.48\pm0.04$&$0.5\pm0.0$&$0.5\pm0.0$&$0.5\pm0.0$\\

& $1$& $0.49\pm0.07$& $0.51\pm0.01$&$0.47\pm0.03$&$0.5\pm0.0$&$0.5\pm0.0$&$0.5\pm0.0$\\

& $2$& $0.48\pm0.1$& $0.52\pm0.01$&$0.49\pm0.03$&$0.5\pm0.0$&$0.5\pm0.0$&$0.5\pm0.0$\\

& $3$& $0.47\pm0.08$& $0.51\pm0.01$&$0.47\pm0.04$&$0.5\pm0.0$&$0.5\pm0.0$&$0.5\pm0.0$\\

& $4$& $0.48\pm0.1$& $0.51\pm0.01$&$0.47\pm0.03$&$0.5\pm0.0$&$0.5\pm0.0$&$0.5\pm0.0$\\

& $5$& $0.51\pm0.11$& $0.52\pm0.01$&$0.5\pm0.01$&$0.5\pm0.0$&$0.5\pm0.0$&$0.5\pm0.0$\\

& $6$& $0.44\pm0.09$& $0.52\pm0.01$&$0.48\pm0.03$&$0.5\pm0.0$&$0.5\pm0.0$&$0.5\pm0.0$\\

& $7$& $0.49\pm0.1$& $0.52\pm0.01$&$0.48\pm0.03$&$0.5\pm0.0$&$0.5\pm0.0$&$0.5\pm0.0$\\

& $8$& $0.5\pm0.09$& $0.52\pm0.0$&$0.48\pm0.02$&$0.5\pm0.0$&$0.5\pm0.0$&$0.5\pm0.0$\\

& $9$& $0.46\pm0.1$& $0.52\pm0.01$&$0.47\pm0.04$&$0.5\pm0.0$&$0.5\pm0.0$&$0.5\pm0.0$\\

& $10$& $0.46\pm0.09$& $0.52\pm0.01$&$0.47\pm0.03$&$0.5\pm0.0$&$0.5\pm0.0$&$0.5\pm0.0$\\

\hline
\end{tabular}
       }
\label{tab:hyperparameters}
       \end{table*}
