# Supplementary material for: LPGNet: Link Private Graph Networks for Node Classification
Source: arXiv:2205.03105 source file (2022-09-07)
Supplement: Supplementary file 15 [file ind_attack_1.tex]

\begin{table*}[th!]
\centering
\caption{Attack in Transductive Setting}
\resizebox{\textwidth}{!}{
\begin{tabular}{c c c c c c c c }
\toprule
Model & Epsilon & \multicolumn{2}{c}{TwitchDE} & \multicolumn{2}{c}{TwitchPTBR} & \multicolumn{2}{c}{TwitchRU}\\\hline
 & & \baselineAttack & \sotaAttack & \baselineAttack & \sotaAttack & \baselineAttack & \sotaAttack\\\hline

\mlp
& $\infty$ & $0.5 \pm 0.01$ & $0.5 \pm 0.0$ & $0.45 \pm 0.01$ & $0.5 \pm 0.0$ & $0.49 \pm 0.03$ & $0.5 \pm 0.0$\\\hline
\gcn
& $\infty$ & $0.54 \pm 0.02$ & $1.0 \pm 0.0$ & $0.57 \pm 0.05$ & $0.99 \pm 0.0$ & $0.52 \pm 0.01$ & $0.99 \pm 0.0$\\\hline
\toola
& $\infty$ & $0.5 \pm 0.02$ & $0.5 \pm 0.0$ & $0.46 \pm 0.02$ & $0.5 \pm 0.0$ & $0.48 \pm 0.01$ & $0.5 \pm 0.0$\\\hline
\toolb
& $\infty$ & $0.5 \pm 0.01$ & $0.5 \pm 0.0$ & $0.45 \pm 0.03$ & $0.5 \pm 0.0$ & $0.48 \pm 0.01$ & $0.5 \pm 0.0$\\\hline

\multirow{10}{*}{\dpgcn}
& $1.0$ & $0.48 \pm 0.02$ & $0.54 \pm 0.02$ & $0.52 \pm 0.02$ & $0.56 \pm 0.01$ & $0.49 \pm 0.02$ & $0.51 \pm 0.03$\\

& $2.0$ & $0.5 \pm 0.03$ & $0.57 \pm 0.01$ & $0.52 \pm 0.02$ & $0.62 \pm 0.0$ & $0.49 \pm 0.02$ & $0.53 \pm 0.04$\\

& $3.0$ & $0.5 \pm 0.02$ & $0.6 \pm 0.03$ & $0.53 \pm 0.02$ & $0.74 \pm 0.02$ & $0.5 \pm 0.02$ & $0.6 \pm 0.04$\\

& $4.0$ & $0.52 \pm 0.01$ & $0.71 \pm 0.01$ & $0.54 \pm 0.03$ & $0.85 \pm 0.01$ & $0.52 \pm 0.02$ & $0.7 \pm 0.03$\\

& $5.0$ & $0.51 \pm 0.02$ & $0.8 \pm 0.01$ & $0.55 \pm 0.04$ & $0.93 \pm 0.01$ & $0.49 \pm 0.02$ & $0.82 \pm 0.02$\\

& $6.0$ & $0.52 \pm 0.02$ & $0.91 \pm 0.01$ & $0.54 \pm 0.03$ & $0.96 \pm 0.01$ & $0.52 \pm 0.02$ & $0.91 \pm 0.01$\\

& $7.0$ & $0.53 \pm 0.02$ & $0.96 \pm 0.01$ & $0.55 \pm 0.01$ & $0.95 \pm 0.0$ & $-1.0 \pm -1.0$ & $-1.0 \pm -1.0$\\

& $8.0$ & $0.52 \pm 0.02$ & $0.97 \pm 0.0$ & $0.57 \pm 0.02$ & $0.98 \pm 0.0$ & $0.54 \pm 0.01$ & $0.97 \pm 0.01$\\

& $9.0$ & $0.55 \pm 0.02$ & $0.98 \pm 0.0$ & $0.55 \pm 0.03$ & $0.98 \pm 0.0$ & $0.52 \pm 0.02$ & $0.98 \pm 0.01$\\

& $10.0$ & $0.54 \pm 0.01$ & $0.99 \pm 0.0$ & $0.57 \pm 0.03$ & $0.98 \pm 0.0$ & $0.52 \pm 0.01$ & $0.99 \pm 0.0$\\
\hline

\multirow{10}{*}{\toola}
& $1.0$ & $0.49 \pm 0.01$ & $0.5 \pm 0.0$ & $0.47 \pm 0.04$ & $0.5 \pm 0.0$ & $0.51 \pm 0.02$ & $0.5 \pm 0.0$\\

& $2.0$ & $0.5 \pm 0.01$ & $0.5 \pm 0.0$ & $0.47 \pm 0.04$ & $0.5 \pm 0.0$ & $0.51 \pm 0.01$ & $0.5 \pm 0.0$\\

& $3.0$ & $0.48 \pm 0.02$ & $0.5 \pm 0.0$ & $0.46 \pm 0.02$ & $0.5 \pm 0.0$ & $0.51 \pm 0.01$ & $0.5 \pm 0.0$\\

& $4.0$ & $0.5 \pm 0.01$ & $0.5 \pm 0.0$ & $0.46 \pm 0.02$ & $0.5 \pm 0.0$ & $0.51 \pm 0.01$ & $0.5 \pm 0.0$\\

& $5.0$ & $0.49 \pm 0.01$ & $0.5 \pm 0.0$ & $0.47 \pm 0.01$ & $0.5 \pm 0.0$ & $0.51 \pm 0.01$ & $0.5 \pm 0.0$\\

& $6.0$ & $0.5 \pm 0.01$ & $0.5 \pm 0.0$ & $0.47 \pm 0.03$ & $0.5 \pm 0.0$ & $0.51 \pm 0.02$ & $0.5 \pm 0.0$\\

& $7.0$ & $0.49 \pm 0.02$ & $0.5 \pm 0.0$ & $0.48 \pm 0.02$ & $0.5 \pm 0.0$ & $0.51 \pm 0.01$ & $0.5 \pm 0.0$\\

& $8.0$ & $0.49 \pm 0.03$ & $0.5 \pm 0.0$ & $0.46 \pm 0.03$ & $0.5 \pm 0.0$ & $0.5 \pm 0.02$ & $0.5 \pm 0.0$\\

& $9.0$ & $0.49 \pm 0.01$ & $0.5 \pm 0.0$ & $0.47 \pm 0.04$ & $0.5 \pm 0.0$ & $0.51 \pm 0.01$ & $0.5 \pm 0.0$\\

& $10.0$ & $0.48 \pm 0.02$ & $0.5 \pm 0.0$ & $0.45 \pm 0.02$ & $0.5 \pm 0.0$ & $0.51 \pm 0.01$ & $0.5 \pm 0.0$\\
\hline

\multirow{10}{*}{\toolb}
& $1.0$ & $0.49 \pm 0.02$ & $0.5 \pm 0.0$ & $0.46 \pm 0.02$ & $0.5 \pm 0.0$ & $0.5 \pm 0.01$ & $0.5 \pm 0.0$\\

& $2.0$ & $-1.0 \pm -1.0$ & $-1.0 \pm -1.0$ & $0.46 \pm 0.03$ & $0.5 \pm 0.0$ & $0.51 \pm 0.01$ & $0.5 \pm 0.0$\\

& $3.0$ & $0.5 \pm 0.02$ & $0.5 \pm 0.0$ & $0.46 \pm 0.03$ & $0.5 \pm 0.0$ & $0.51 \pm 0.02$ & $0.5 \pm 0.0$\\

& $4.0$ & $0.5 \pm 0.01$ & $0.5 \pm 0.0$ & $0.47 \pm 0.02$ & $0.5 \pm 0.0$ & $0.51 \pm 0.01$ & $0.5 \pm 0.0$\\

& $5.0$ & $0.5 \pm 0.01$ & $0.5 \pm 0.0$ & $0.46 \pm 0.02$ & $0.5 \pm 0.0$ & $0.51 \pm 0.01$ & $0.5 \pm 0.0$\\

& $6.0$ & $0.5 \pm 0.02$ & $0.5 \pm 0.0$ & $0.45 \pm 0.03$ & $0.5 \pm 0.0$ & $0.51 \pm 0.01$ & $0.5 \pm 0.0$\\

& $7.0$ & $0.49 \pm 0.02$ & $0.5 \pm 0.0$ & $0.45 \pm 0.03$ & $0.5 \pm 0.0$ & $0.51 \pm 0.01$ & $0.5 \pm 0.0$\\

& $8.0$ & $0.5 \pm 0.02$ & $0.5 \pm 0.0$ & $0.46 \pm 0.03$ & $0.5 \pm 0.0$ & $0.51 \pm 0.02$ & $0.5 \pm 0.0$\\

& $9.0$ & $0.5 \pm 0.02$ & $0.5 \pm 0.0$ & $0.45 \pm 0.04$ & $0.5 \pm 0.0$ & $0.51 \pm 0.02$ & $0.5 \pm 0.0$\\

& $10.0$ & $0.5 \pm 0.02$ & $0.5 \pm 0.0$ & $0.47 \pm 0.02$ & $0.5 \pm 0.0$ & $0.51 \pm 0.02$ & $0.5 \pm 0.0$\\
\hline

\end{tabular}
}
\label{tab:ind_1_attack}
\end{table*}
