# Supplementary material for: LPGNet: Link Private Graph Networks for Node Classification
Source: arXiv:2205.03105 source file (2022-09-07)
Supplement: Supplementary file 17 [file utility_attack_efficient_pubmed.tex]

\nextgroupplot[title style={yshift=-1.2ex},
title={\pubmed, \sotaAttack}
]
\addplot+[scatter,
    only marks,
    scatter/classes={MMLP_nl1={mark=triangle,red},
                     MMLP_nl2={mark=triangle,red},
                     gcn={mark=o,blue},
                     mlp={mark=+,black},
                     nondp-gcn={mark=+,brown}
                    },
  scatter src=explicit symbolic,
  ] table[x=f1_score_mean, y=auc_score_mean, meta=model]\loadedtableEfficientPubMed;

\addplot[color = black, dashed, thick] coordinates {(0.5474,0.5) (0.7915,0.5)};
  \addplot[color = black, dashed, thick] coordinates {(0.7292,-1.0) (0.7292, 0.9999)};
  \addplot[color = brown, dashed, thick] coordinates {(0.5474,0.9999) (0.7915,0.9999)};
  \addplot[color = brown, dashed, thick] coordinates {(0.7915,-1.0) (0.7915, 0.9999)};
   \draw [fill=gray,gray,fill opacity=0.4] (axis cs:0.7292,0.5) rectangle (axis cs:0.7915,0.9999);
